# Supplementary material for: AdaTyper: Adaptive Semantic Column Type Detection
Source: arXiv:2311.13806 source file (2023-11-23)
Supplement: Supplementary file 1 [file 09_appendix.tex]

\appendix

\section{Semantic types}

\madelon{This might be converted into a distribution and combined with Figure~\ref{fig:annotation-distribution}}

\begin{table*}[h]
    \centering
    \caption{Semantic types and categories that \system is trained and evaluated on.}
    \begin{tabular}{l l c c }
    \toprule
    \textbf{Category} & \textbf{type} & \textbf{Number samples GitTables (train)} & \textbf{Number samples human-annotated CTU PRLR (test)} \\
    \hline
    \multirow{10}{*}{Geographic} & \type{continent} & & \\
    & \type{state} & & \\
    & \type{county} & & \\
    & \type{country} & & \\
    & \type{country code} & & \\
    & \type{city} & & \\
    & \type{postal code} & & \\
    & \type{address} & & \\
    & \type{latitude} & & \\
    & \type{longitude} & & \\
    \hline
    \multirow{4}{*}{Temporal} & \type{date} & & \\
    & \type{year} & & \\
    & \type{month} & & \\
    & \type{week} & & \\
    \hline
    \multirow{6}{*}{Personal} & \type{first name} & & \\
    & \type{last name} & & \\
    & \type{age} & & \\
    & \type{gender} & & \\
    & \type{email} & & \\
    & \type{phone number} & & \\
    \hline
    \multirow{6}{*}{Business} & \type{id} & & \\
    & \type{company name} & & \\
    & \type{product} & & \\
    & \type{price} & & \\
    & \type{currency} & & \\
    & \type{percentage} & & \\
    \bottomrule
    \end{tabular}
    \label{tab:semantic-types}
\end{table*}
